# Supplementary material for: Measuring the Performance and Network Utilization of Popular Video Conferencing Applications
Source: arXiv:2105.13478 source file (2021-05-27)
Supplement: Supplementary file 1 [file appendix.tex]

\newpage
\appendix
\thispagestyle{plain}
\section{Additional Plots and Tables}

\FloatBarrier

\setcounter{figure}{0}

\setcounter{table}{0}

\begin{figure}[!b]
    \centering
    \includegraphics[width=\linewidth]{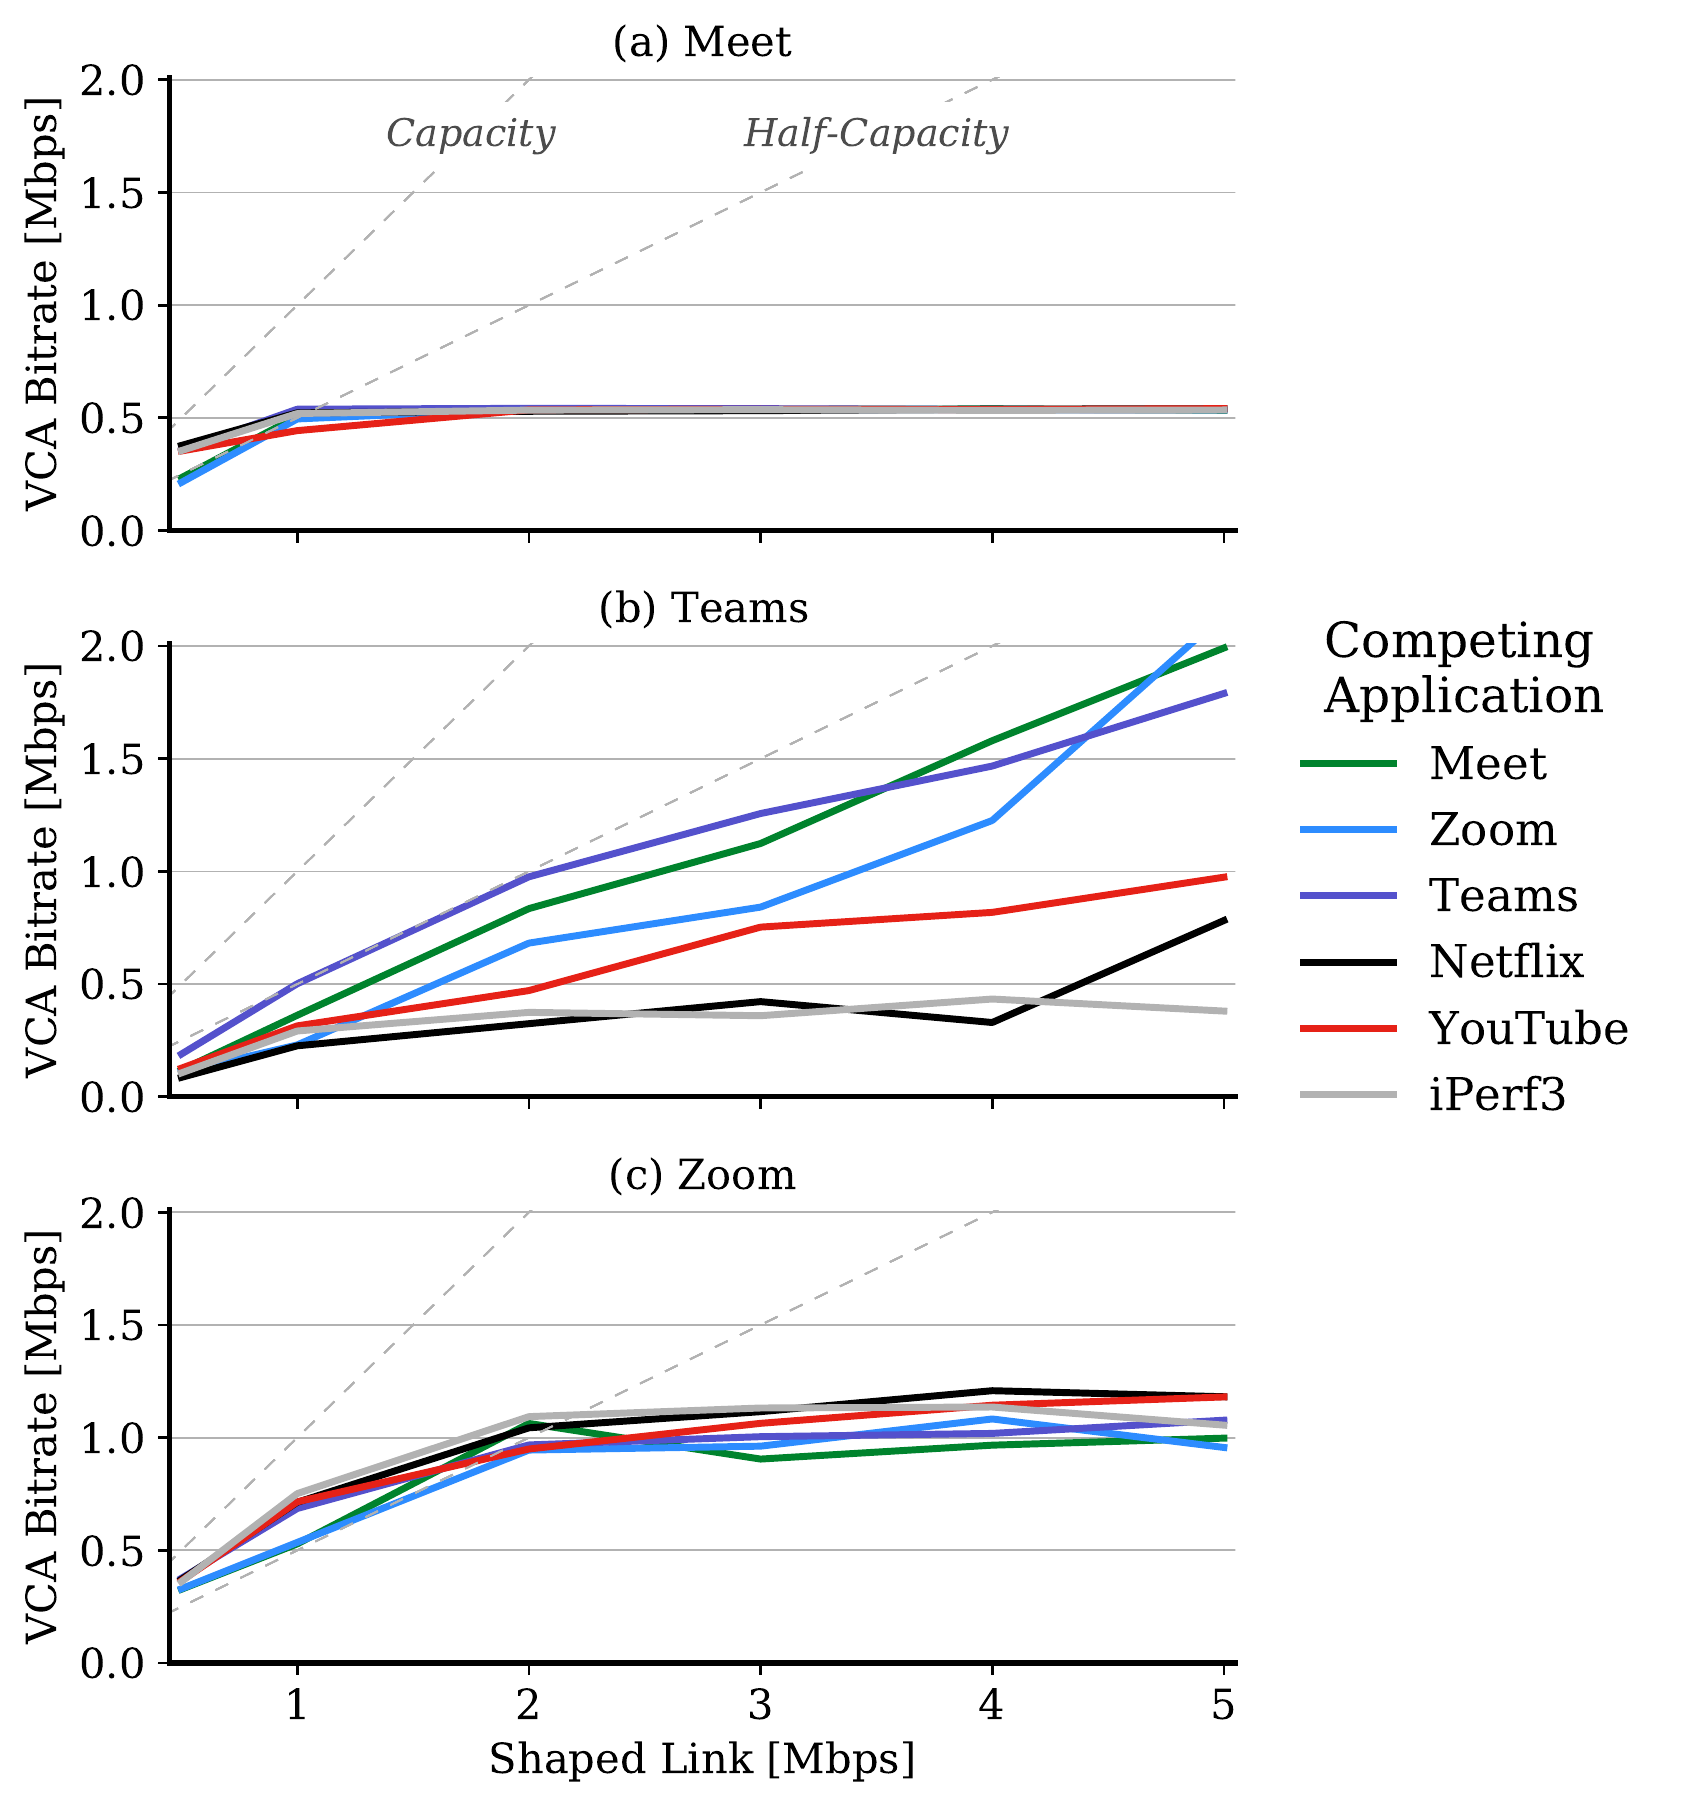}
    \caption{VCA bitrates on a constrained downstream link, shared with other applications.  The figure labels (a-c) denote the incumbent flow, and the lines its consumption.}
    \label{fig:comp_dl}
\end{figure}
